# Supplementary material for: Privacy Preserving Multi Agent Path Finding
Source: arXiv:2605.14119 source file (2026-05-13)
Supplement: Supplementary file 1 [file supplementary_material.tex]

%%%% For anonymized submission, use this
% \documentclass[sigconf,anonymous]{aamas} 

%%%% For camera-ready, use this
\documentclass[sigconf]{aamas} 

%%% Load required packages here (note that many are included already).
\usepackage{balance} % for balancing columns on the final page

\usepackage{graphicx} % Required for inserting images
\usepackage{hyperref}
\usepackage{caption}
\usepackage[ruled,vlined,linesnumbered]{algorithm2e}
\usepackage{xcolor}
\usepackage{subcaption}
\usepackage{natbib}
\usepackage{multirow}
\usepackage{footnote}
\usepackage{amsmath}
\usepackage{amsthm}
\usepackage{booktabs}
\usepackage{xspace}
\usepackage{tabularx}

\captionsetup{compatibility=false}

\renewcommand{\cite}{\citep}

% CPPP stuff:

% MAPF stuff:

\newcommand{\ekppmapf}{\textsc {ekPPMAPF}\xspace}
\newcommand{\fpp}{\textsc {fPP}\xspace}
\newcommand{\ppfpp}{\textsc {PPfPP}\xspace}

\newcommand{\commentout}[1]{}

\SetKwProg{Fn}{Function}{:}{end}
\SetKwProg{Cls}{Class}{:}{end}
\SetKw{Params}{Parameters:}
\SetKwRepeat{DoWhile}{do}{while}

\commentout{
\newtheorem{myclaim}{myclaim}

\newtheorem{theorem}{Theorem}

\newtheoremstyle{exampstyle}
  {-.25pt} % Space above
  {-.25pt} % Space below
  {\itshape} % Body font
  {} % Indent amount
  {\bfseries} % Theorem head font
  {.} % Punctuation after theorem head
  {.5em} % Space after theorem head
  {} % Theorem head spec (can be left empty, meaning `normal')
\theoremstyle{exampstyle}
}
\newtheorem{theorem}{Theorem}
\newtheorem{definition}{Definition}

\newcommand{\plan}[1]{ }

\newcommand{\rotem}[1]{}
\newcommand{\roni}[1]{}
\newcommand{\guy}[1]{}

% \newcommand{\rotem}[1]{ }
% \newcommand{\roni}[1]{ }
% \newcommand{\guy}[1]{ }

%%%%%%%%%%%%%%%%%%%%%%%%%%%%%%%%%%%%%%%%%%%%%%%%%%%%%%%%%%%%%%%%%%%%%%%%

%%% AAMAS-2026 copyright block (do not change!)

\setcopyright{ifaamas}
\acmConference[AAMAS '26]{Proc.\@ of the 25th International Conference
on Autonomous Agents and Multiagent Systems (AAMAS 2026)}{May 25 -- 29, 2026}
{Paphos, Cyprus}{C.~Amato, L.~Dennis, V.~Mascardi, J.~Thangarajah (eds.)}
\copyrightyear{2026}
\acmYear{2026}
\acmDOI{}
\acmPrice{}
\acmISBN{}

%%%%%%%%%%%%%%%%%%%%%%%%%%%%%%%%%%%%%%%%%%%%%%%%%%%%%%%%%%%%%%%%%%%%%%%%

%%% == IMPORTANT ==
%%% Use this command to specify your submission number.
%%% In anonymous mode, it will be printed on the first page.

\acmSubmissionID{823}

%%% Use this command to specify the title of your paper.

\title[Privacy Preserving MAPF - Supplementary Material]{Privacy Preserving Multi Agent Path Finding - Supplementary Material}

%%% Provide names, affiliations, and email addresses for all authors.

\author{Rotem Lev Lehman}
\affiliation{
  \institution{Ben Gurion University of the Negev}
  \city{Be'er Sheva}
  \country{Israel}}
\email{levlerot@post.bgu.ac.il}

\author{Roni Stern}
\affiliation{
  \institution{Ben Gurion University of the Negev}
  \city{Be'er Sheva}
  \country{Israel}}
\email{sternron@bgu.ac.il}

\author{Guy Shani}
\affiliation{
  \institution{Ben Gurion University of the Negev}
  \city{Be'er Sheva}
  \country{Israel}}
\email{shanigu@bgu.ac.il}

\newcommand{\BibTeX}{\rm B\kern-.05em{\sc i\kern-.025em b}\kern-.08em\TeX}

%%%%%%%%%%%%%%%%%%%%%%%%%%%%%%%%%%%%%%%%%%%%%%%%%%%%%%%%%%%%%%%%%%%%%%%%

\begin{document}

%%% The following commands remove the headers in your paper. For final 
%%% papers, these will be inserted during the pagination process.

\pagestyle{fancy}
\fancyhead{}

%%% The next command prints the information defined in the preamble.

\maketitle 

%%%%%%%%%%%%%%%%%%%%%%%%%%%%%%%%%%%%%%%%%%%%%%%%%%%%%%%%%%%%%%%%%%%%%%%%

\section{Theorems and Proofs for \ppfpp}

\begin{definition}[Initial Safe-Zone]
    \label{def:initial-safe-zone}
    The initial safe-zone of an agent group $a_i$ in a specific timestep $t$ on a given plan $\Pi$ that was generated from running \fpp on an \ekppmapf problem P, denoted $IS_i^t(\Pi)$, is the set $\{v | F_i(v) \subseteq FoV_i^t(\Pi)\}$.
\end{definition}

\begin{definition}[Agent Group's FoV]
    \label{def:agent-group-fov}
    An agent group $a_i$'s FoV in timestep $t$ on a given plan $\Pi$ generated by \fpp on an \ekppmapf problem P, denoted $FoV_i^t(\Pi)$, is the set $\{v | \exists a_{i_j} v \in F_i(\Pi_j(t))\}$.
\end{definition}

\begin{definition}[Runtime k-Privacy]
    \label{def:runtime-k-privacy}
    A MAPF solution $\Pi$ preserves \emph{Runtime k-Privacy} if 
    the belief state generated from finding $\Pi$ preserves k-Privacy and there are no $FoV$ conflicts in $\Pi$.
\end{definition}

\begin{definition}[Separated Safe Zones]
    \label{def:safe-zone-safeness}
    A set of safe-zones $S(\Pi) = \left\{ S_i(\Pi) | \forall i \in A \right\}$, is called separated, if and only if: \\$\forall{t}\forall{i \in A} \forall{v \in S_i^t(\Pi)} \forall{j \neq i} \nexists{u \in S_j^t(\Pi)}: u \in F_i(v) || v \in F_j(u)$.
\end{definition}

\begin{algorithm}[b!]
		\caption{Post-Processing (\fpp) Solutions (\ppfpp)}
            \label{alg:ppfpp}
            \SetKw{KwInput}{Input:}
            \SetKw{KwOutput}{Output:}
            
            \KwInput{$\Pi$: An \ekppmapf solution}\\
            \KwOutput{$\Pi'$ refined for all agent groups}
            
		\Fn{PPfPP}{
                $IS(\Pi) \gets \text{initial safe zone as defined in definition~\ref{def:initial-safe-zone}}$ \;
                $ES(\Pi)\gets ExtendSafeZone(IS(\Pi))$ \;
                \label{line:ppfpp-es}
                \ForEach{$a_i \in A$}{
                    $a_i.FindPathForRealAgent(ES_i(\Pi))$ \;
                }
            }

            \Fn{ExtendSafeZone(IS)}{
                \label{line:ppfpp-extend-safe-zone}
                ES $\gets$ IS  \;
                \label{line:ppfpp-extend-safe-zone-initialize}

                \ForEach{$t \in T$}{
                    \DoWhile{$\neg done$}{
                        $done \gets TRUE$\;
                        \ForEach{$a_i \in A$}{
                            \label{line:alg_ppfpp_extend_safe_zone__foreach_agent}
                            $picked \gets a_i.ExtendSafeZone(ES^t)$  \;
                            \label{line:ppfpp-a_i-extend-safe-zone}
                            $done \gets done \land \neg picked$  \;
                        }
                    }
                }
                \Return ES \;
            }

\end{algorithm}

\begin{definition}[Rules for Extending Safe Zone]
    \label{def:rules-for-extended-safe-zone}
    The function $a_i.ExtendSafeZone(ES^t)$ is a function that $a_i$ uses for extending the safe zone $ES_i^t$. It must pick one vertex $v$ to add to $ES_i^t$. It returns $TRUE$ if found $v$ that was added to $ES_i^t$, $FALSE$ otherwise, and it must follow the following rules:
    \begin{enumerate}
        \item $v$ is a neighbor of some $u \in ES_i^t$.
        \item $\forall a_j, v \notin ES_j^t$.
        \label{item:rules-for-extended-safe-zone--es-unique}
        \item $\forall a_j \neq a_i, \nexists u \in ES_j^t: u \in F_i(v) \| v \in F_j(u)$.
        \label{item:rules-for-extended-safe-zone--out-of-fov}
        \item Using it must preserve the runtime k-Privacy of $\mu,\Pi$ after running it.
    \end{enumerate}
\end{definition}

\plan{Theorem for safeness}

\begin{theorem}[Initial safe-Zone Safeness]
    \label{theorem:initial-safe-zone-safeness}
    An initial safe-zone $IS(\Pi)$ calculated from definition~\ref{def:initial-safe-zone}, when $\forall a_i, a_j \in A \forall v \in V: F_i(v)=F_j(v) \And F_i \text{ is symmetric}$, is safe.
\end{theorem}

\begin{proof}
    Given an \ekppmapf problem P, a valid plan $\Pi$ that solves P, and was returned by using \fpp on P, an initial safe-zone $IS(\Pi)$ calculated from definition~\ref{def:initial-safe-zone}, and $\forall a_i, a_j \in A \forall v \in V: F_i(v)=F_j(v) \And F_i \text{ is symmetric}$.
    Let $a_i, a_j \in A| a_i \neq a_j, t \in T$.
    Also, let $v \in IS_i^t(\Pi)$.
    Assume negatively that $\exists u \in IS_j^t: \left( u \in F_i(v) \| v \in F_j(u) \right)$, without loss of generality, assume $u \in F_i(v)$.
    From definition~\ref{def:initial-safe-zone}, $u \in FoV_i^t(\Pi)$, hence from definition~\ref{def:agent-group-fov}, $\exists a_{i_p}: u \in F_i(\Pi_p(t))$, because that $F_i$ is symmetric, $\Rightarrow \Pi_p(t) \in F_i(u)$ and because $F_i = F_j \Rightarrow \Pi_p(t) \in F_j(u)$. Because of $u \in IS_j^t(\Pi)$, then $F_j(u) \subseteq FoV_j^t(\Pi) \Rightarrow \Pi_p(t) \in FoV_j^t(\Pi)$, and so from definition~\ref{def:agent-group-fov}, $\exists a_{j_q}: \Pi_p(t) \in F_j(\Pi_q(t))$. But $a_{i_p}$ and $a_{j_q}$ are of different agent groups, and so this is a FoV conflict $\Rightarrow$ from definition~\ref{def:runtime-k-privacy}, $\Pi$ does $not$ preserve Runtime k-Privacy, and so $\Pi$ is not a valid \ekppmapf plan, in contradiction to the assumption that $\Pi$ is a valid plan that solves P.
    $\Rightarrow \nexists u \in IS_j^t: \left( u \in F_i(v) \| v \in F_j(u) \right) \Rightarrow$ from definition~\ref{def:safe-zone-safeness} $IS(\Pi)$ is considered safe.
\end{proof}

\begin{theorem}[Extended Safe-Zone Safeness]
    \label{theorem:extended-safe-zone-safeness}
    An extended safe-zone $ES(\Pi)$ calculated from running $ExtendSafeZone$ in line~\ref{line:ppfpp-extend-safe-zone} in algorithm~\ref{alg:ppfpp} on $IS$ calculated from definition~\ref{def:initial-safe-zone}, when the function $a_i.ExtendSafeZone(ES^t)$ from line~\ref{line:ppfpp-a_i-extend-safe-zone} follows the rules from definition~\ref{def:rules-for-extended-safe-zone}, when $\forall a_i, a_j \in A \forall v \in V: F_i(v)=F_j(v) \And F_i \text{ is symmetric}$, is safe.
\end{theorem}

\plan{Proof for safeness}

\begin{proof}
    Given an \ekppmapf problem P, a valid plan $\Pi$ that solves P, and was returned by using \fpp on P, an extended safe-zone $ES(\Pi)$ calculated from running $ExtendSafeZone$, where the function $a_i.ExtendSafeZone(ES^t)$ from line~\ref{line:ppfpp-a_i-extend-safe-zone} follows the rules from definition~\ref{def:rules-for-extended-safe-zone}, and $\forall a_i, a_j \in A \forall v \in V: F_i(v)=F_j(v) \And F_i \text{ is symmetric}$.
    Let $a_i, a_j \in A| a_i \neq a_j, t \in T$.
    Also, let $v \in ES_i^t(\Pi), u \in ES_j^t(\Pi)$.
    There are four possible cases:
    \begin{itemize}
        \item $v \in IS_i^t(\Pi) \And u \in IS_j^t(\Pi)$: From theorem~\ref{theorem:initial-safe-zone-safeness} and definition~\ref{def:safe-zone-safeness}, $u \notin F_i(v) \And v \notin F_j(u)$.
        \item $v \in IS_i^t(\Pi) \And u \notin IS_j^t(\Pi)$: So in line~\ref{line:ppfpp-a_i-extend-safe-zone} in algorithm~\ref{alg:ppfpp}, there was some iteration where $u$ was added to $ES_j^t$. In this iteration we called $a_i.ExtendSafeZone(ES^t)$ where $IS_i^t \subseteq ES_i^t$, since it was set at line~\ref{line:ppfpp-extend-safe-zone-initialize} to be $IS_i^t$, and $u \notin ES_j^t$ since it was added in this iteration to $ES_j^t$. From definition~\ref{def:rules-for-extended-safe-zone}, rule number~\ref{item:rules-for-extended-safe-zone--out-of-fov} we can conclude that $u \notin F_i(v) \And v \notin F_j(u)$.
        \item $v \notin IS_i^t(\Pi) \And u \in IS_j^t(\Pi)$: Same as the previous case.
        \item $v \notin IS_i^t(\Pi) \And u \notin IS_j^t(\Pi)$: So, without loss of generality, there was an iteration in line~\ref{line:ppfpp-a_i-extend-safe-zone} in algorithm~\ref{alg:ppfpp}, where $v$ was added to $ES_i^t$, and $u$ was not yet added to $ES_j^t$. This iteration is the same as the previous case, and so $u \notin F_i(v) \And v \notin F_j(u)$.
    \end{itemize}
    As you can see, in all cases $u \notin F_i(v) \And v \notin F_j(u) \Rightarrow$ from definition~\ref{def:safe-zone-safeness} $ES(\Pi)$ is considered safe.
\end{proof}

\plan{Theorem for \ppfpp returning valid \ekppmapf plans}

\begin{theorem}[\ppfpp Solves \ekppmapf Problems]
    \label{theorem:ppfpp-solves-ekppmapf}
    If $ES$ was calculated using a $a_i.ExtendSafeZone(ES^t)$ function that follows the rules from definition~\ref{def:rules-for-extended-safe-zone}, and $\forall a_i, a_j \in A \forall v \in V: F_i(v)=F_j(v) \And F_i \text{ is symmetric} \And \forall u \in v.neighbors: u \in F_i(v)$, then \ppfpp returns valid \ekppmapf plans.
\end{theorem}

\plan{Proof for valid plans}

\balance
\begin{proof}
\sloppy{
    Given that $ES$ in algorithm~\ref{alg:ppfpp} is calculated using a $a_i.ExtendSafeZone(ES^t)$ function that follows the rules from definition~\ref{def:rules-for-extended-safe-zone}, and $\forall a_i, a_j \in A \forall v \in V: F_i(v)=F_j(v) \And F_i \text{ is symmetric} \And \forall u \in v.neighbors: u \in F_i(v)$.
    Also given an \ekppmapf problem P, a plan $\Pi$ originated from running the \fpp algorithm, and a plan $\Pi'$ that returned from running \ppfpp on $\Pi$.
    From theorem~\ref{theorem:extended-safe-zone-safeness} we can conclude that $ES(\Pi)$ is safe. So $\forall a_i \in A$, if we find a plan for $a_i.real\_agent$ that stays only in the safe-zone $ES_i$, it will not conflict with any other $a_j \neq a_i$ in the FoV. Also, there will be no $vertex$ conflicts, because of rule number~\ref{item:rules-for-extended-safe-zone--es-unique} in definition~\ref{def:rules-for-extended-safe-zone}. Let $a_i, a_j \in A: a_i \neq a_j$ assume negatively that $\exists t \in T:$ there is a swapping conflict between $a_i$ and $a_j$ in $\Pi'$ on time steps $t-1, t$. Let $v$ be the vertex $a_i$ is at time $t-1$ on $\Pi'$ and $u$ be the vertex $a_j$ is at time $t-1$ on $Pi'$. From the assumptions ($\forall a_i\in A \forall v \in V \forall u \in v.neighbors: u \in F_i(v)$), $\Rightarrow u \in F_i(v) \And v \in F_j(u) \Rightarrow$ in time $t-1$ there is a $FoV$ conflict - but we proved (in this proof) that there are no $FoV$ conflicts, so there is a contradiction, $\Rightarrow \nexists t \in T:$ there is a swapping conflict between $a_i$ and $a_j$ in $\Pi'$ on time steps $t-1, t \Rightarrow$ there are no $swapping$ conflicts in the resulting plan $\Pi'$. So $\Pi'$ is a valid plan for P.}
\end{proof}

\section{Experimental Results}

In this section we show all experimental results not shown in the main paper.
Trends are the same as in the main paper and so are not discussed here.

%%%%%%%%%%%%%%%%%%%%%%%%%%%%%%%%%%%%%%%%%%%%% All results for fpp run to be copied to the supplimentry material %%%%%%%%%%%%%%%%%%%%%%%

%%%%%%%%%%%%%%% fpp figures: %%%%%%%%%%%%%%%%

%k figure:
\begin{figure*}[t]
\centering
\begin{subfigure}[t]{0.20\textwidth}
\centering
  \includegraphics[width=1\linewidth]{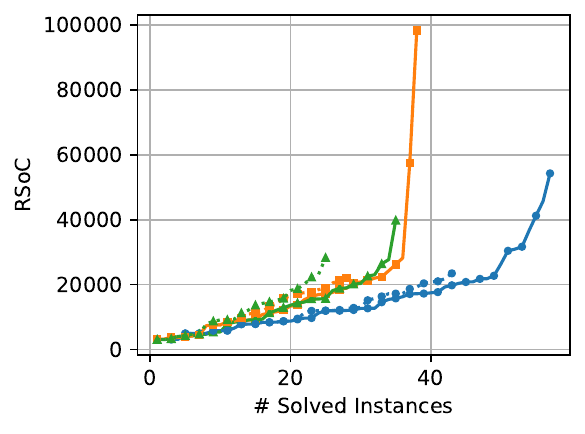}
  \caption{$brc202d$}
  \label{fig:fpp_k__brc202d}
  \Description{Cactus chart of RSoC for each configuration of k in each sub-solver (LaCAM/PIBT) over \# of solved instances for the map brc202d.}
\end{subfigure}\hspace{1em}
\begin{subfigure}[t]{0.20\textwidth}
\centering
  \includegraphics[width=1\linewidth]{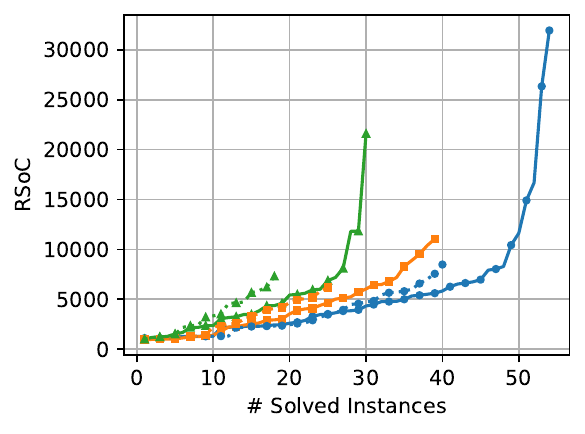}
  \caption{$lt\_gallowstemplar\_n$}
  \label{fig:fpp_k__lt_gallowstemplar_n}
  \Description{Cactus chart of RSoC for each configuration of k in each sub-solver (LaCAM/PIBT) over \# of solved instances for the map lt_gallowstemplar_n.}
\end{subfigure}\hspace{1em}
\begin{subfigure}[t]{0.20\textwidth}
\centering
  \includegraphics[width=1\linewidth]{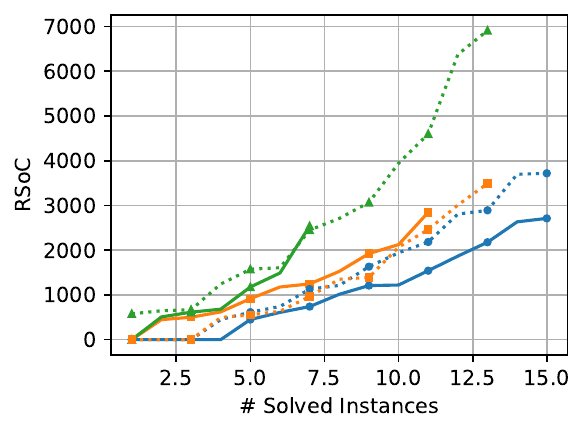}
  \caption{$maze-32-32-2$}
  \label{fig:fpp_k__maze-32-32-2}
  \Description{Cactus chart of RSoC for each configuration of k in each sub-solver (LaCAM/PIBT) over \# of solved instances for the map maze-32-32-2.}
\end{subfigure}\hspace{1em}
\begin{subfigure}[t]{0.20\textwidth}
\centering
  \includegraphics[width=1\linewidth]{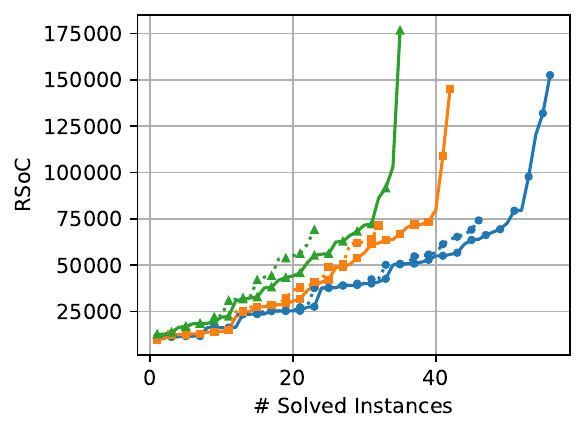}
  \caption{$orz900d$}
  \label{fig:fpp_k__orz900d}
  \Description{Cactus chart of RSoC for each configuration of k in each sub-solver (LaCAM/PIBT) over \# of solved instances for the map orz900d.}
\end{subfigure}\hspace{1em}
\begin{subfigure}[t]{0.20\textwidth}
\centering
  \includegraphics[width=1\linewidth]{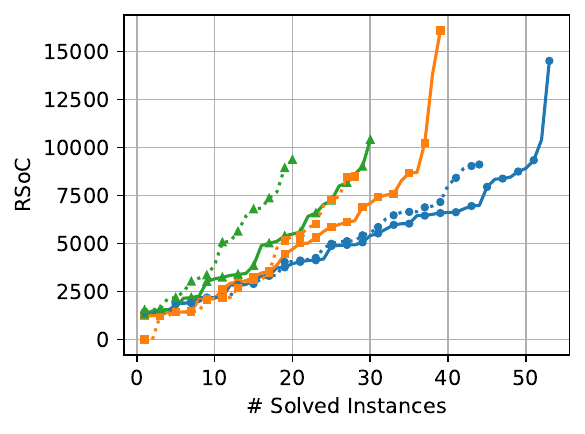}
  \caption{$ost003d$}
  \label{fig:fpp_k__ost003d}
  \Description{Cactus chart of RSoC for each configuration of k in each sub-solver (LaCAM/PIBT) over \# of solved instances for the map ost003d.}
\end{subfigure}\hspace{1em}
\begin{subfigure}[t]{0.20\textwidth}
\centering
  \includegraphics[width=1\linewidth]{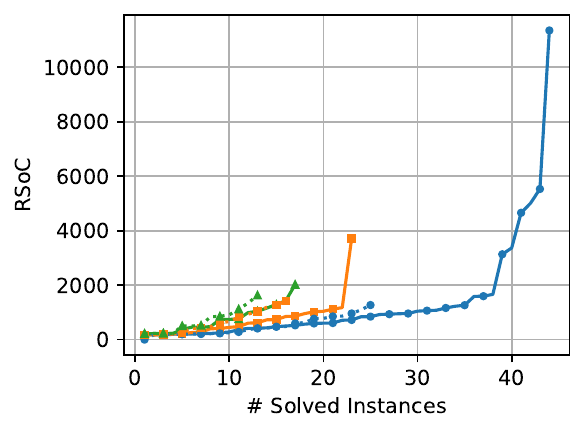}
  \caption{$random-32-32-20$}
  \label{fig:fpp_k__random-32-32-20}
  \Description{Cactus chart of RSoC for each configuration of k in each sub-solver (LaCAM/PIBT) over \# of solved instances for the map random-32-32-20.}
\end{subfigure}\hspace{1em}
\begin{subfigure}[t]{0.20\textwidth}
\centering
  \includegraphics[width=1\linewidth]{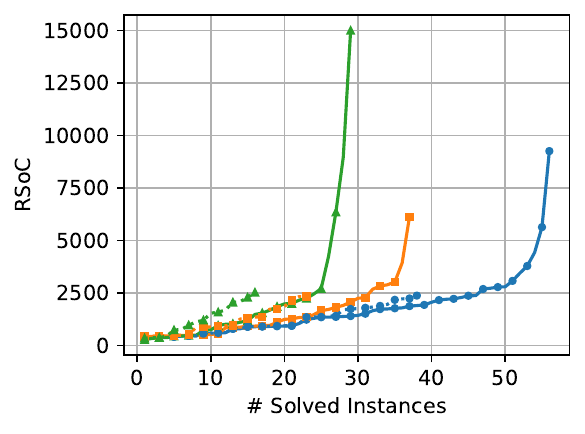}
  \caption{$random-64-64-20$}
  \label{fig:fpp_k__random-64-64-20}
  \Description{Cactus chart of RSoC for each configuration of k in each sub-solver (LaCAM/PIBT) over \# of solved instances for the map random-64-64-20.}
\end{subfigure}\hspace{1em}
\begin{subfigure}[t]{0.20\textwidth}
\centering
  \includegraphics[width=1\linewidth]{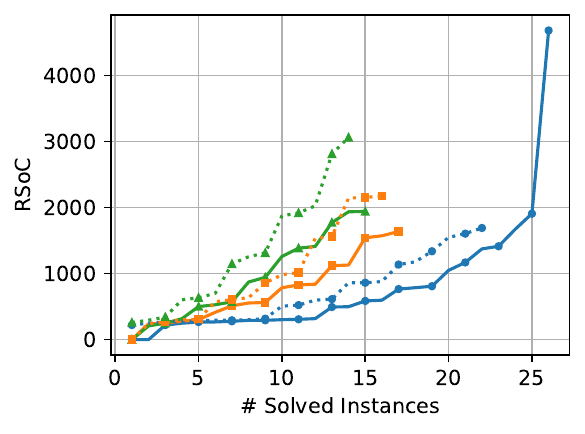}
  \caption{$room-32-32-4$}
  \label{fig:fpp_k__room-32-32-4}
  \Description{Cactus chart of RSoC for each configuration of k in each sub-solver (LaCAM/PIBT) over \# of solved instances for the map room-32-32-4.}
\end{subfigure}\hspace{1em}
\begin{subfigure}[t]{0.20\textwidth}
\centering
  \includegraphics[width=1\linewidth]{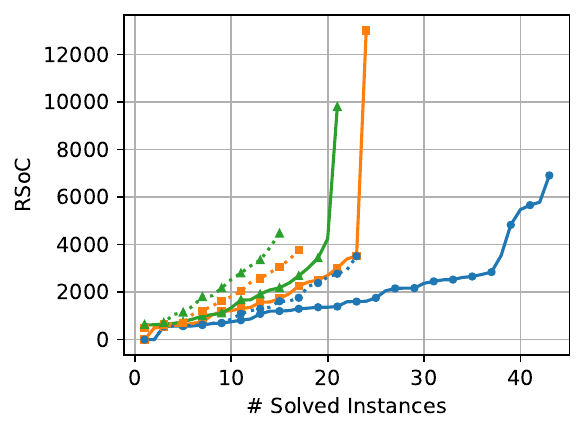}
  \caption{$room-64-64-8$}
  \label{fig:fpp_k__room-64-64-8}
  \Description{Cactus chart of RSoC for each configuration of k in each sub-solver (LaCAM/PIBT) over \# of solved instances for the map room-64-64-8.}
\end{subfigure}\hspace{1em}
\begin{subfigure}[t]{0.20\textwidth}
\centering
  \includegraphics[width=1\linewidth]{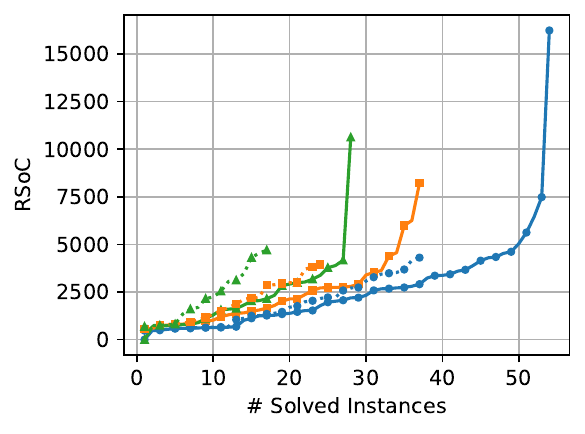}
  \caption{$room-64-64-16$}
  \label{fig:fpp_k__room-64-64-16}
  \Description{Cactus chart of RSoC for each configuration of k in each sub-solver (LaCAM/PIBT) over \# of solved instances for the map room-64-64-16.}
\end{subfigure}\hspace{1em}
\begin{subfigure}[t]{0.20\textwidth}
\centering
  \includegraphics[width=1\linewidth]{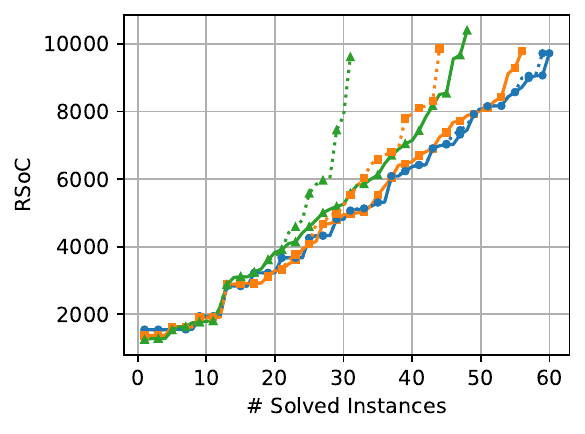}
  \caption{$warehouse-20-40-10-2-1$}
  \label{fig:fpp_k__warehouse-20-40-10-2-1}
  \Description{Cactus chart of RSoC for each configuration of k in each sub-solver (LaCAM/PIBT) over \# of solved instances for the map warehouse-20-40-10-2-1.}
\end{subfigure}\hspace{1em}
\begin{subfigure}[t]{0.20\textwidth}
\centering
  \includegraphics[width=1\linewidth]{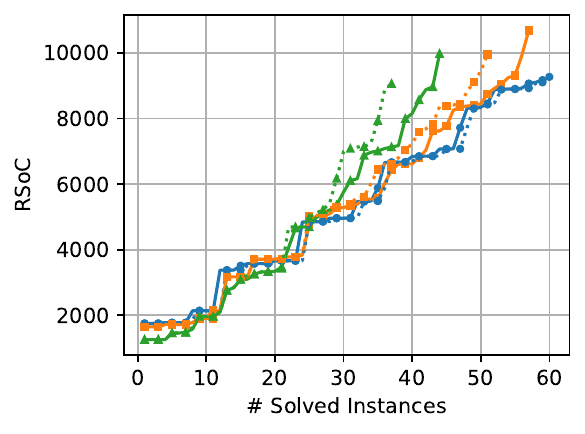}
  \caption{$warehouse-20-40-10-2-2$}
  \label{fig:fpp_k__warehouse-20-40-10-2-2}
  \Description{Cactus chart of RSoC for each configuration of k in each sub-solver (LaCAM/PIBT) over \# of solved instances for the map warehouse-20-40-10-2-2.}
\end{subfigure}\hspace{1em}
% Second row for the shared legend
\begin{minipage}{\textwidth}
    \centering
    \includegraphics[width=0.7\linewidth]{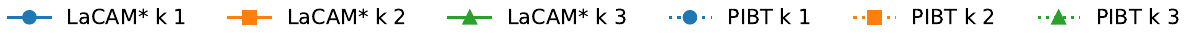}
    \label{fig:fpp_k__legend}
    \Description{Legend}
\end{minipage}
\caption{Cactus chart of $RSoC$ for each configuration of $k$ in each sub-solver $(LaCAM/PIBT)$ over \# of solved instances.}
\label{fig:fpp_k}
\end{figure*}

%FoV figure:
\begin{figure*}[t]
\centering
\begin{subfigure}[t]{0.20\textwidth}
\centering
  \includegraphics[width=1\linewidth]{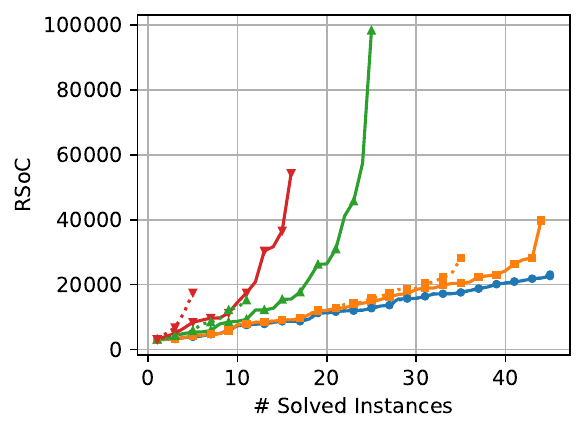}
  \caption{$brc202d$}
  \label{fig:fpp_fov__brc202d}
  \Description{Cactus chart of RSoC for each configuration of FoV in each sub-solver (LaCAM/PIBT) over \# of solved instances for the map brc202d.}
\end{subfigure}\hspace{1em}
\begin{subfigure}[t]{0.20\textwidth}
\centering
  \includegraphics[width=1\linewidth]{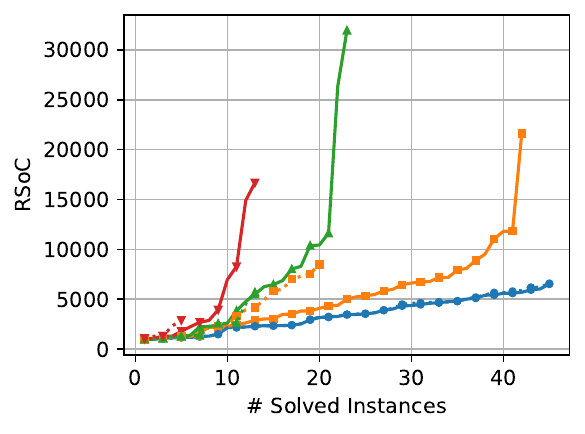}
  \caption{$lt\_gallowstemplar\_n$}
  \label{fig:fpp_fov__lt_gallowstemplar_n}
  \Description{Cactus chart of RSoC for each configuration of FoV in each sub-solver (LaCAM/PIBT) over \# of solved instances for the map lt_gallowstemplar_n.}
\end{subfigure}\hspace{1em}
\begin{subfigure}[t]{0.20\textwidth}
\centering
  \includegraphics[width=1\linewidth]{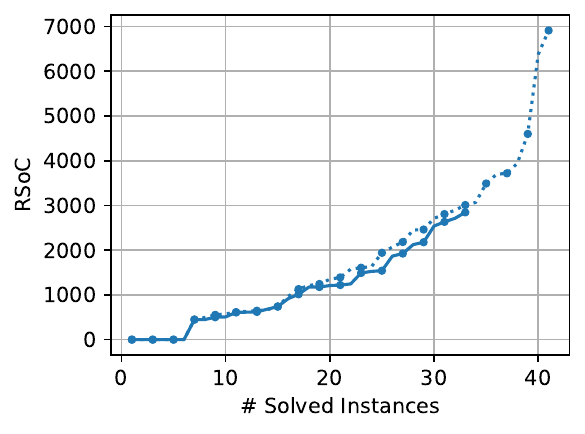}
  \caption{$maze-32-32-2$}
  \label{fig:fpp_fov__maze-32-32-2}
  \Description{Cactus chart of RSoC for each configuration of FoV in each sub-solver (LaCAM/PIBT) over \# of solved instances for the map maze-32-32-2.}
\end{subfigure}\hspace{1em}
\begin{subfigure}[t]{0.20\textwidth}
\centering
  \includegraphics[width=1\linewidth]{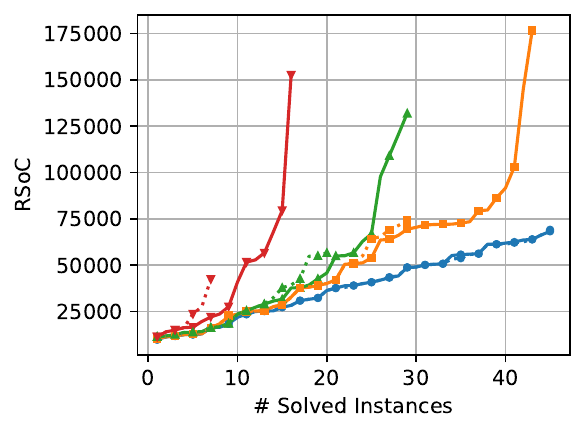}
  \caption{$orz900d$}
  \label{fig:fpp_fov__orz900d}
  \Description{Cactus chart of RSoC for each configuration of FoV in each sub-solver (LaCAM/PIBT) over \# of solved instances for the map orz900d.}
\end{subfigure}\hspace{1em}
\begin{subfigure}[t]{0.20\textwidth}
\centering
  \includegraphics[width=1\linewidth]{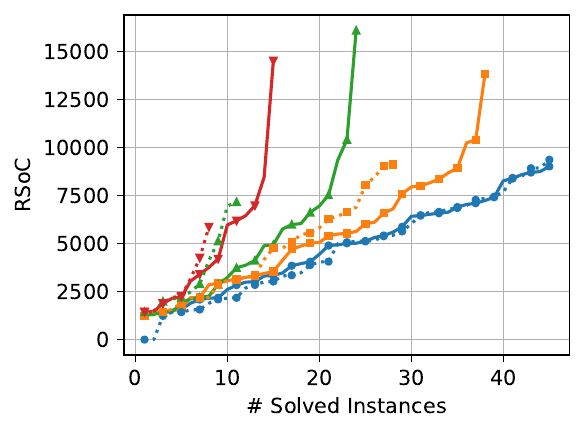}
  \caption{$ost003d$}
  \label{fig:fpp_fov__ost003d}
  \Description{Cactus chart of RSoC for each configuration of FoV in each sub-solver (LaCAM/PIBT) over \# of solved instances for the map ost003d.}
\end{subfigure}\hspace{1em}
\begin{subfigure}[t]{0.20\textwidth}
\centering
  \includegraphics[width=1\linewidth]{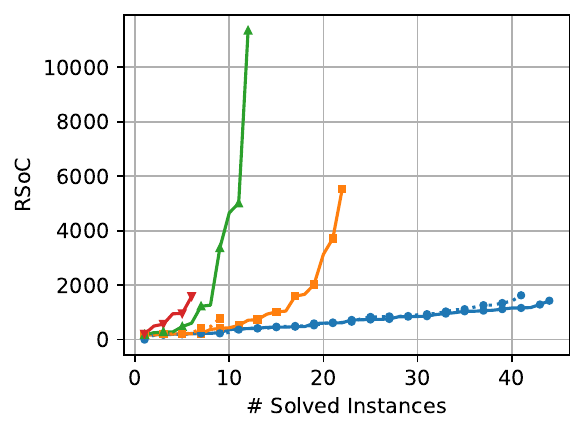}
  \caption{$random-32-32-20$}
  \label{fig:fpp_fov__random-32-32-20}
  \Description{Cactus chart of RSoC for each configuration of FoV in each sub-solver (LaCAM/PIBT) over \# of solved instances for the map random-32-32-20.}
\end{subfigure}\hspace{1em}
\begin{subfigure}[t]{0.20\textwidth}
\centering
  \includegraphics[width=1\linewidth]{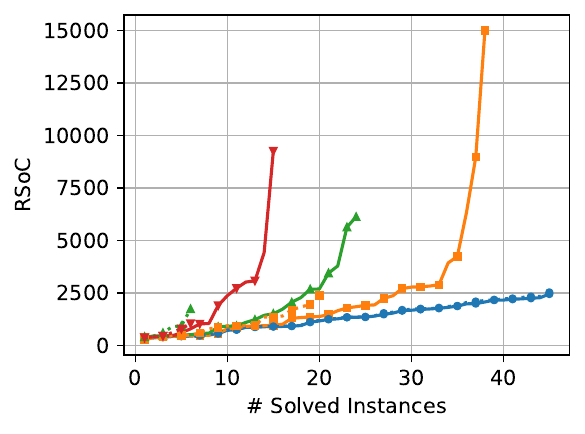}
  \caption{$random-64-64-20$}
  \label{fig:fpp_fov__random-64-64-20}
  \Description{Cactus chart of RSoC for each configuration of FoV in each sub-solver (LaCAM/PIBT) over \# of solved instances for the map random-64-64-20.}
\end{subfigure}\hspace{1em}
\begin{subfigure}[t]{0.20\textwidth}
\centering
  \includegraphics[width=1\linewidth]{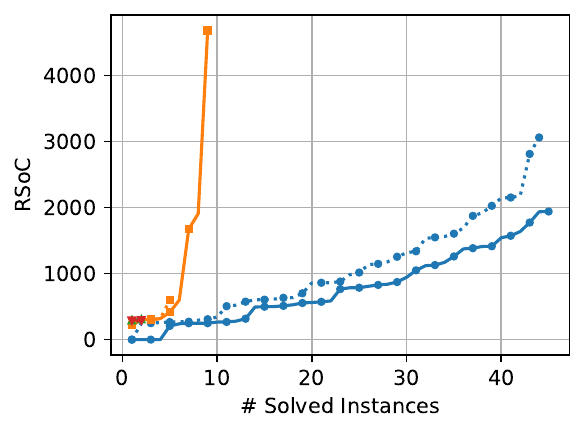}
  \caption{$room-32-32-4$}
  \label{fig:fpp_fov__room-32-32-4}
  \Description{Cactus chart of RSoC for each configuration of FoV in each sub-solver (LaCAM/PIBT) over \# of solved instances for the map room-32-32-4.}
\end{subfigure}\hspace{1em}
\begin{subfigure}[t]{0.20\textwidth}
\centering
  \includegraphics[width=1\linewidth]{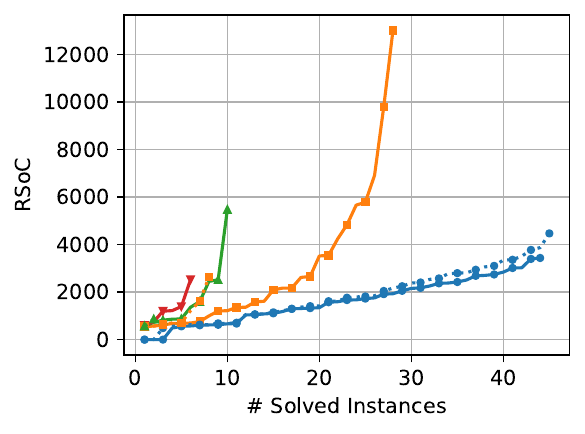}
  \caption{$room-64-64-8$}
  \label{fig:fpp_fov__room-64-64-8}
  \Description{Cactus chart of RSoC for each configuration of FoV in each sub-solver (LaCAM/PIBT) over \# of solved instances for the map room-64-64-8.}
\end{subfigure}\hspace{1em}
\begin{subfigure}[t]{0.20\textwidth}
\centering
  \includegraphics[width=1\linewidth]{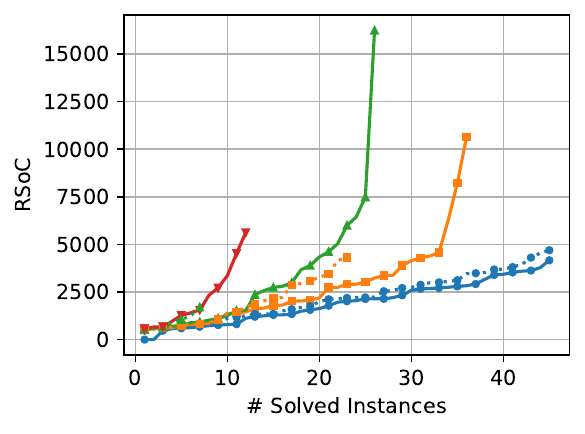}
  \caption{$room-64-64-16$}
  \label{fig:fpp_fov__room-64-64-16}
  \Description{Cactus chart of RSoC for each configuration of FoV in each sub-solver (LaCAM/PIBT) over \# of solved instances for the map room-64-64-16.}
\end{subfigure}\hspace{1em}
\begin{subfigure}[t]{0.20\textwidth}
\centering
  \includegraphics[width=1\linewidth]{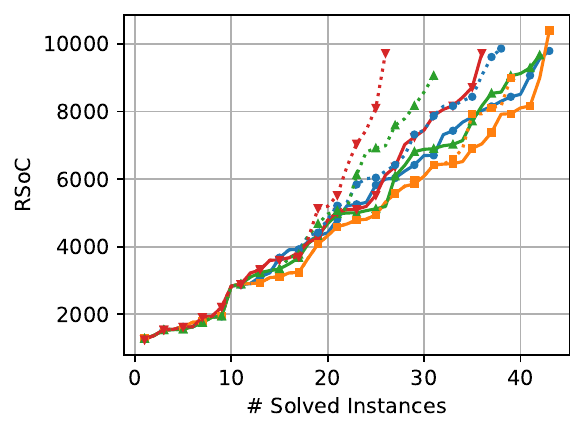}
  \caption{$warehouse-20-40-10-2-1$}
  \label{fig:fpp_fov__warehouse-20-40-10-2-1}
  \Description{Cactus chart of RSoC for each configuration of FoV in each sub-solver (LaCAM/PIBT) over \# of solved instances for the map warehouse-20-40-10-2-1.}
\end{subfigure}\hspace{1em}
\begin{subfigure}[t]{0.20\textwidth}
\centering
  \includegraphics[width=1\linewidth]{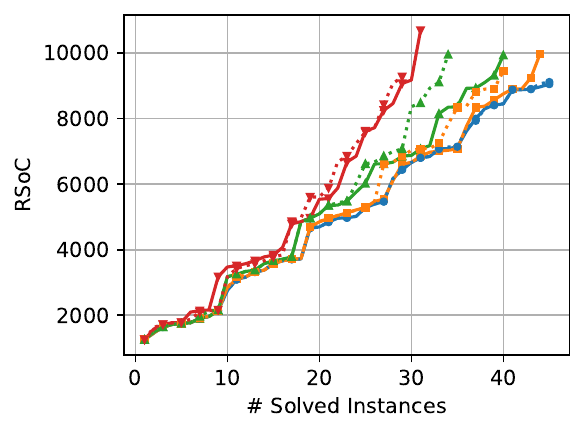}
  \caption{$warehouse-20-40-10-2-2$}
  \label{fig:fpp_fov__warehouse-20-40-10-2-2}
  \Description{Cactus chart of RSoC for each configuration of FoV in each sub-solver (LaCAM/PIBT) over \# of solved instances for the map warehouse-20-40-10-2-2.}
\end{subfigure}\hspace{1em}
% Second row for the shared legend
\begin{minipage}{\textwidth}
    \centering
    \includegraphics[width=0.9\linewidth]{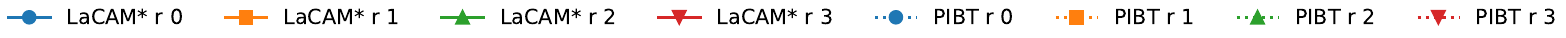}
    \label{fig:fpp_fov__legend}
    \Description{Legend}
\end{minipage}
\caption{Cactus chart of $RSoC$ for each configuration of $FoV$ in each sub-solver $(LaCAM/PIBT)$ over \# of solved instances.}
\label{fig:fpp_fov}
\end{figure*}

\commentout{
\begin{figure*}[ht]
    \includegraphics[width=\linewidth]{ppfpp_results/ppfpp.pdf}
    \caption{A heatmap for each of the following metrics: \emph{RSoC improvement \%} $\left(\frac{RSoC(fPP)-RSoC(PPfPP)}{RSoC(fPP)}\right)*100\%$, \emph{\ppfpp runtime $[s]$} and \emph{\fpp makespan}. In the \emph{RSoC improvement \%} heatmap, * and ** marks significant improvement of \ppfpp over \fpp (Wilcoxon, p $<$ 0.05 and p $<$ 0.01 accordingly). Each heatmap's y axis is the map we run on and the x axis is the k value we run on. Each map shows the size of the map in vertices ($|V|$). A mean over all maps is also shown. The results here are for both sub-solvers PIBT and LaCAM$^*$ together.
    }
    \label{fig:ppfpp_results}
    \Description{Results for the \ppfpp algorithm improving the \fpp output in terms of RSoC. Presenting 3 heatmaps 1 for each metric \emph{RSoC improvement \%}, \emph{\ppfpp runtime $[s]$} and \emph{\fpp makespan}.}
\end{figure*}
}

\begin{table*}[ht]
\caption[\ppfpp improves \fpp RSoC]{Average \emph{RSoC improvement\%} $\left(\frac{RSoC(fPP)-RSoC(PPfPP)}{RSoC(fPP)}\right)*100\%$ (mean $\pm$ std, max and median (med)) of \ppfpp over \fpp, across domains with different k values. \#S is the amount of solved instances by \fpp (all instances also were also solved by \ppfpp). * and ** marks significant improvement of \ppfpp over \fpp (Wilcoxon, p $<$ 0.05 and p $<$ 0.01 accordingly). \fpp MS is the makespan of the original plan created by \fpp. Each map shows the amount of vertices in it $(|V|)$.
This table contains part of the maps we ran on, and the other part is in the second table~\ref{tab:ppfpp-rsoc2} which also contains the mean over all maps.}
\label{tab:ppfpp-rsoc}
\begin{tabular}{llllllll}
\toprule
Map & k & \multicolumn{3}{c}{$RSoC \ Improvement\%$} & \#S & time & \fpp \\
 &  & mean $\pm$ std & max & med &  & [s] & MS \\
\midrule
\multirow[c]{9}{*}{\shortstack{brc202d\\$|V|=43{,}151$}} & $2$ & $0.77 \pm 2.47^{**}$ & $11.50$ & $0.02$ & $56$ & $113.6$ & $943.9$ \\
 & $3$ & $0.64 \pm 1.65^{**}$ & $7.25$ & $0.02$ & $55$ & $116.0$ & $975.4$ \\
 & $4$ & $1.04 \pm 2.69^{**}$ & $11.30$ & $0.02$ & $47$ & $121.2$ & $1022.4$ \\
 & $5$ & $1.06 \pm 2.66^{**}$ & $11.27$ & $0.00$ & $40$ & $125.3$ & $1041.3$ \\
 & $6$ & $1.20 \pm 2.68^{**}$ & $10.72$ & $0.02$ & $39$ & $124.0$ & $1040.9$ \\
 & $7$ & $1.80 \pm 3.90^{**}$ & $12.90$ & $0.03$ & $42$ & $131.0$ & $1094.5$ \\
 & $8$ & $2.04 \pm 4.45^{**}$ & $16.91$ & $0.07$ & $30$ & $137.6$ & $1170.1$ \\
 & $9$ & $3.21 \pm 6.40^{**}$ & $22.83$ & $0.11$ & $25$ & $143.4$ & $1203.6$ \\
 & $10$ & $1.01 \pm 2.69^{**}$ & $13.21$ & $0.07$ & $25$ & $143.8$ & $1312.6$ \\
\cline{1-8}
\multirow[c]{9}{*}{\shortstack{$\text{lt\_gallowstemplar\_n}$\\$|V|=10{,}021$}} & $2$ & $0.64 \pm 1.66^{**}$ & $8.23$ & $0.00$ & $59$ & $3.2$ & $245.2$ \\
 & $3$ & $0.88 \pm 1.77^{**}$ & $8.02$ & $0.14$ & $50$ & $3.2$ & $270.3$ \\
 & $4$ & $0.24 \pm 0.84^{**}$ & $5.60$ & $0.07$ & $45$ & $3.3$ & $284.4$ \\
 & $5$ & $0.87 \pm 1.65^{**}$ & $5.14$ & $0.14$ & $34$ & $3.7$ & $316.6$ \\
 & $6$ & $0.74 \pm 1.75^{**}$ & $7.20$ & $0.15$ & $24$ & $3.9$ & $348.0$ \\
 & $7$ & $0.70 \pm 2.51^{**}$ & $12.87$ & $0.09$ & $26$ & $3.8$ & $342.4$ \\
 & $8$ & $0.89 \pm 2.06^{**}$ & $9.54$ & $0.26$ & $21$ & $4.8$ & $421.0$ \\
 & $9$ & $2.06 \pm 3.43^{**}$ & $10.30$ & $0.36$ & $12$ & $5.0$ & $418.8$ \\
 & $10$ & $0.45 \pm 1.13^{**}$ & $4.03$ & $0.15$ & $12$ & $5.9$ & $508.2$ \\
\cline{1-8}
\multirow[c]{9}{*}{\shortstack{ost003d\\$|V|=13{,}214$}} & $2$ & $0.59 \pm 1.84^{**}$ & $8.83$ & $0.00$ & $52$ & $7.2$ & $346.6$ \\
 & $3$ & $1.19 \pm 3.14^{**}$ & $13.15$ & $0.05$ & $49$ & $7.0$ & $363.9$ \\
 & $4$ & $0.68 \pm 1.88^{**}$ & $9.27$ & $0.04$ & $40$ & $6.9$ & $375.8$ \\
 & $5$ & $1.22 \pm 2.86^{**}$ & $10.38$ & $0.06$ & $30$ & $7.9$ & $410.8$ \\
 & $6$ & $2.13 \pm 4.02^{**}$ & $17.06$ & $0.15$ & $30$ & $7.5$ & $401.2$ \\
 & $7$ & $1.29 \pm 2.45^{**}$ & $6.89$ & $0.13$ & $18$ & $7.8$ & $427.9$ \\
 & $8$ & $2.20 \pm 4.54^{**}$ & $16.25$ & $0.15$ & $14$ & $9.7$ & $518.4$ \\
 & $9$ & $2.49 \pm 3.75^{**}$ & $10.33$ & $0.20$ & $14$ & $9.0$ & $461.8$ \\
 & $10$ & $0.10 \pm 0.06^{**}$ & $0.17$ & $0.11$ & $8$ & $12.9$ & $665.5$ \\
\cline{1-8}
\multirow[c]{5}{*}{\shortstack{$\text{random-32-32-20}$\\$|V|=819$}} & $2$ & $0.64 \pm 1.38^{**}$ & $4.83$ & $0.00$ & $43$ & $0.0$ & $48.3$ \\
 & $3$ & $2.14 \pm 3.51^{**}$ & $10.66$ & $0.41$ & $30$ & $0.1$ & $61.5$ \\
 & $4$ & $0.78 \pm 0.84^{**}$ & $3.33$ & $0.50$ & $19$ & $0.1$ & $108.5$ \\
 & $5$ & $1.73 \pm 2.66^{**}$ & $8.38$ & $0.41$ & $11$ & $0.1$ & $192.6$ \\
 & $6$ & $0.14 \pm 0.13$ & $0.25$ & $0.16$ & $4$ & $0.2$ & $286.5$ \\
\cline{1-8}
\multirow[c]{9}{*}{\shortstack{$\text{random-64-64-20}$\\$|V|=3{,}270$}} & $2$ & $0.20 \pm 1.05^{**}$ & $7.75$ & $0.00$ & $56$ & $0.3$ & $90.5$ \\
 & $3$ & $0.62 \pm 1.89^{**}$ & $10.34$ & $0.00$ & $48$ & $0.3$ & $96.7$ \\
 & $4$ & $0.73 \pm 1.84^{**}$ & $7.65$ & $0.00$ & $38$ & $0.3$ & $100.3$ \\
 & $5$ & $1.33 \pm 2.60^{**}$ & $10.00$ & $0.23$ & $29$ & $0.4$ & $106.8$ \\
 & $6$ & $1.04 \pm 2.30^{**}$ & $8.33$ & $0.20$ & $21$ & $0.4$ & $120.4$ \\
 & $7$ & $0.70 \pm 1.24^{**}$ & $4.85$ & $0.19$ & $19$ & $0.4$ & $146.4$ \\
 & $8$ & $0.93 \pm 1.88^{**}$ & $5.72$ & $0.23$ & $15$ & $0.5$ & $151.8$ \\
 & $9$ & $2.97 \pm 5.36^{**}$ & $18.32$ & $0.16$ & $12$ & $0.7$ & $244.6$ \\
 & $10$ & $0.86 \pm 1.55^*$ & $3.64$ & $0.16$ & $5$ & $0.9$ & $294.6$ \\
\cline{1-8}
\multirow[c]{2}{*}{\shortstack{$\text{room-32-32-4}$\\$|V|=682$}} & $2$ & $1.17 \pm 1.61^{**}$ & $4.32$ & $0.29$ & $28$ & $0.0$ & $65.2$ \\
 & $3$ & $0.93 \pm 2.08^{**}$ & $6.84$ & $0.32$ & $10$ & $0.1$ & $123.9$ \\
\cline{1-8}

\bottomrule
\end{tabular}
\end{table*}

\begin{table*}[ht]
\caption[\ppfpp improves \fpp RSoC]{Average \emph{RSoC improvement\%} $\left(\frac{RSoC(fPP)-RSoC(PPfPP)}{RSoC(fPP)}\right)*100\%$ (mean $\pm$ std, max and median (med)) of \ppfpp over \fpp, across domains with different k values. \#S is the amount of solved instances by \fpp (all instances also were also solved by \ppfpp). * and ** marks significant improvement of \ppfpp over \fpp (Wilcoxon, p $<$ 0.05 and p $<$ 0.01 accordingly). \fpp MS is the makespan of the original plan created by \fpp. Each map shows the amount of vertices in it $(|V|)$.
This is a complementary table for the rest of the maps not shown in table~\ref{tab:ppfpp-rsoc} including the mean over all maps.}
\label{tab:ppfpp-rsoc2}
\begin{tabular}{llllllll}
\toprule
Map & k & \multicolumn{3}{c}{$RSoC \ Improvement\%$} & \#S & time & \fpp \\
 &  & mean $\pm$ std & max & med &  & [s] & MS \\
\midrule
\multirow[c]{9}{*}{\shortstack{$\text{room-64-64-16}$\\$|V|=3{,}646$}} & $2$ & $0.95 \pm 2.47^{**}$ & $11.21$ & $0.00$ & $56$ & $0.6$ & $164.0$ \\
 & $3$ & $1.06 \pm 3.73^{**}$ & $25.74$ & $0.14$ & $50$ & $0.5$ & $172.4$ \\
 & $4$ & $0.50 \pm 0.98^{**}$ & $3.51$ & $0.11$ & $36$ & $0.6$ & $180.5$ \\
 & $5$ & $1.80 \pm 3.98^{**}$ & $19.11$ & $0.19$ & $27$ & $0.7$ & $196.7$ \\
 & $6$ & $1.13 \pm 2.45^{**}$ & $11.09$ & $0.11$ & $22$ & $0.8$ & $242.2$ \\
 & $7$ & $2.76 \pm 5.64^{**}$ & $18.33$ & $0.24$ & $12$ & $0.9$ & $258.7$ \\
 & $8$ & $2.02 \pm 3.53^{**}$ & $9.80$ & $0.33$ & $11$ & $0.8$ & $239.5$ \\
 & $9$ & $0.08 \pm 0.11$ & $0.15$ & $0.08$ & $2$ & $1.1$ & $300.5$ \\
 & $10$ & $0.11 \pm 0.08$ & $0.21$ & $0.10$ & $4$ & $2.2$ & $635.5$ \\
\cline{1-8}
\multirow[c]{6}{*}{\shortstack{$\text{room-64-64-8}$\\$|V|=3{,}232$}} & $2$ & $0.32 \pm 1.11^{**}$ & $6.93$ & $0.00$ & $51$ & $0.3$ & $125.6$ \\
 & $3$ & $0.13 \pm 0.14^{**}$ & $0.38$ & $0.11$ & $34$ & $0.4$ & $144.9$ \\
 & $4$ & $0.56 \pm 1.68^{**}$ & $8.02$ & $0.17$ & $22$ & $0.5$ & $182.4$ \\
 & $5$ & $0.66 \pm 1.29^{**}$ & $3.94$ & $0.13$ & $16$ & $0.6$ & $241.9$ \\
 & $6$ & $0.19 \pm 0.19^*$ & $0.45$ & $0.06$ & $5$ & $0.8$ & $350.2$ \\
 & $7$ & $0.11 \pm nan$ & $0.11$ & $0.11$ & $1$ & $0.5$ & $197.0$ \\
\cline{1-8}
\multirow[c]{9}{*}{\shortstack{$\text{warehouse-20-40-10-2-1}$\\$|V|=22{,}599$}} & $2$ & $0.00 \pm 0.01^*$ & $0.08$ & $0.00$ & $59$ & $11.5$ & $341.2$ \\
 & $3$ & $0.00 \pm 0.01$ & $0.05$ & $0.00$ & $59$ & $11.1$ & $348.7$ \\
 & $4$ & $0.00 \pm 0.02^*$ & $0.08$ & $0.00$ & $56$ & $11.2$ & $361.3$ \\
 & $5$ & $0.26 \pm 1.25^{**}$ & $9.03$ & $0.00$ & $57$ & $11.4$ & $367.8$ \\
 & $6$ & $0.34 \pm 1.17^{**}$ & $4.91$ & $0.00$ & $55$ & $11.5$ & $374.7$ \\
 & $7$ & $0.67 \pm 2.16^{**}$ & $10.98$ & $0.00$ & $50$ & $11.9$ & $386.5$ \\
 & $8$ & $0.27 \pm 1.06^{**}$ & $4.99$ & $0.00$ & $50$ & $11.9$ & $384.4$ \\
 & $9$ & $0.99 \pm 2.39^{**}$ & $9.29$ & $0.00$ & $49$ & $12.7$ & $408.0$ \\
 & $10$ & $0.95 \pm 2.14^{**}$ & $9.29$ & $0.00$ & $50$ & $12.4$ & $404.5$ \\
\cline{1-8}
\multirow[c]{9}{*}{\shortstack{$\text{warehouse-20-40-10-2-2}$\\$|V|=38{,}756$}} & $2$ & $0.05 \pm 0.22^*$ & $1.07$ & $0.00$ & $58$ & $41.7$ & $377.2$ \\
 & $3$ & $0.04 \pm 0.17^{**}$ & $1.11$ & $0.00$ & $55$ & $40.3$ & $389.1$ \\
 & $4$ & $0.32 \pm 1.27^{**}$ & $6.97$ & $0.00$ & $57$ & $36.2$ & $392.9$ \\
 & $5$ & $0.63 \pm 1.75^{**}$ & $8.65$ & $0.00$ & $45$ & $34.6$ & $397.6$ \\
 & $6$ & $0.19 \pm 0.60^{**}$ & $2.65$ & $0.00$ & $44$ & $35.1$ & $406.7$ \\
 & $7$ & $0.35 \pm 1.46^{**}$ & $8.31$ & $0.00$ & $34$ & $37.2$ & $428.3$ \\
 & $8$ & $0.75 \pm 1.73^{**}$ & $7.41$ & $0.00$ & $35$ & $39.7$ & $455.7$ \\
 & $9$ & $0.16 \pm 0.65^{**}$ & $3.11$ & $0.00$ & $23$ & $38.3$ & $437.3$ \\
 & $10$ & $0.02 \pm 0.03^*$ & $0.12$ & $0.00$ & $15$ & $35.9$ & $434.6$ \\
\cline{1-8}
\multirow[c]{9}{*}{$\text{Mean}$} & $2$ & $0.50 \pm 1.61^{**}$ & $11.50$ & $0.00$ & $518$ & $19.5$ & $293.3$ \\
 & $3$ & $0.68 \pm 2.22^{**}$ & $25.74$ & $0.00$ & $440$ & $22.3$ & $336.9$ \\
 & $4$ & $0.49 \pm 1.55^{**}$ & $11.30$ & $0.00$ & $360$ & $24.6$ & $374.7$ \\
 & $5$ & $0.93 \pm 2.35^{**}$ & $19.11$ & $0.02$ & $289$ & $26.4$ & $408.3$ \\
 & $6$ & $0.83 \pm 2.25^{**}$ & $17.06$ & $0.00$ & $244$ & $30.2$ & $451.8$ \\
 & $7$ & $1.04 \pm 2.86^{**}$ & $18.33$ & $0.03$ & $202$ & $37.7$ & $507.6$ \\
 & $8$ & $1.06 \pm 2.78^{**}$ & $16.91$ & $0.04$ & $176$ & $36.2$ & $518.6$ \\
 & $9$ & $1.66 \pm 3.90^{**}$ & $22.83$ & $0.05$ & $137$ & $38.6$ & $548.7$ \\
 & $10$ & $0.71 \pm 1.93^{**}$ & $13.21$ & $0.05$ & $119$ & $41.5$ & $630.2$ \\
\cline{1-8}
\bottomrule
\end{tabular}
\end{table*}

% \bibliographystyle{ACM-Reference-Format} 
% \bibliography{main}

%%%%%%%%%%%%%%%%%%%%%%%%%%%%%%%%%%%%%%%%%%%%%%%%%%%%%%%%%%%%%%%%%%%%%%%%

\end{document}
